# Supplementary material for: Electronic bandstructure of superconducting KTaO3 (111) interfaces
Source: arXiv:2311.08230 source file (2023-11-14)
Supplement: Supplementary file 1 [file supplementary.pdf]

## Supplementary Material

# Electronic band structure of superconducting $KTaO_3$ (111) interfaces

Srijani Mallik,[1, a)] Börge Göbel,[2, a)] Hugo Witt,[1, 3, a)] Luis M. Vicente-Arche,[1] Sara Varotto,[1] Julien Bréhin,[1] Gerbold Ménard,[3] Guilhem Saïz,[3] Dyhia Tamsaout,[1] Andrés Felipe Santander-Syro,[4] Franck Fortuna,[4] François Bertran,[5] Patrick Le Fèvre,[5] Julien Rault,[5] Isabella Boventer,[1] Ingrid Mertig,[2] Agnès Barthélémy,[1] Nicolas Bergeal,[3] Annika Johansson,[6] and Manuel Bibes[1]

[1)]Unité Mixte de Physique, CNRS, Thales, Université Paris-Saclay, 91767 Palaiseau, France

[2)]Institute of Physics, Martin-Luther-Universität Halle-Wittenberg, 06099 Halle, Germany

[3)]Laboratoire de Physique et d'Etude des Matériaux, ESPCI Paris, Université PSL, CNRS, 75005, Paris, France

[4)]Institut des Sciences Moléculaires d'Orsay, CNRS, Université Paris-Saclay, 91405 Orsay, France

[5)]SOLEIL synchrotron, L'Orme des Merisiers, Départementale 128, F-91190 Saint-Aubin, France

[6)]Max Planck Institute of Microstructure Physics, Weinberg 2, 06120 Halle, Germany

## Transport measurements:

We prepared two identical samples, one for the ARPES measurement and another with an extra capping layer of 2.1 nm Al for the ex-situ transport measurement. Fig. S1(a) shows the temperature dependence of the sheet resistance of the $2^{nd}$ sample measured just after the ARPES measurement. The sample exhibits metallic behavior with a superconducting $T_c$ of ~1 K. The hall measurement at 2 K revealed the carrier density of the sample to be $11.4 \times 10^{13}$ $cm^{-2}$.

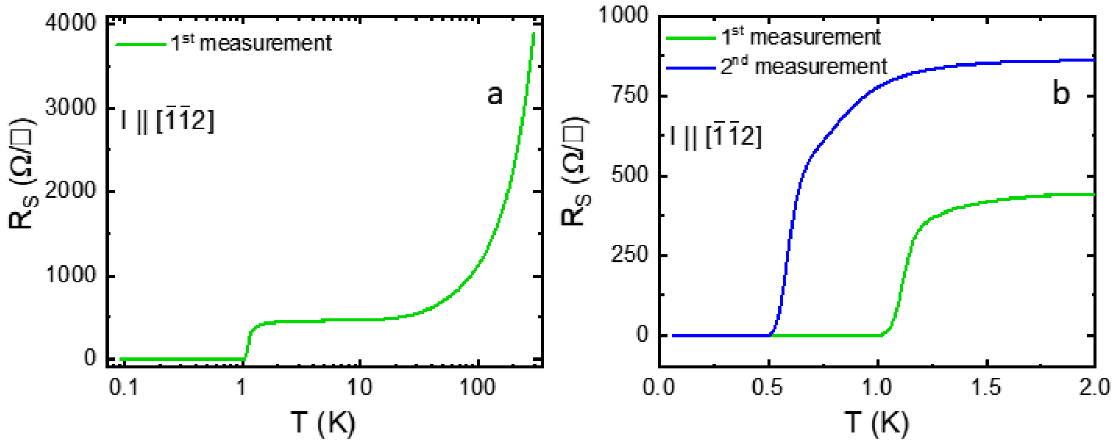


FIG. S1. Temperature dependence of the sheet resistance measured with current parallel to [$\bar{1}\bar{1}2$] (a) just after the ARPES measurement. The data shows metallic behavior from room temperature to 1 K and subsequently a superconducting transition at ~1 K. (b) Comparison of low temperature sheet resistance measurements with current along [$\bar{1}\bar{1}2$] direction just after the ARPES measurement (green solid line) and after one year of the ARPES measurement (blue solid line).

Further, the same sample was measured after one year to check the stability of the two-dimensional electron gas (2DEG) with respect to time. We found that the 2DEG which is formed due to oxygen vacancies got slightly re-oxygenated by air. Consequently, the resistance of the 2DEG increased (Fig. S1(b)) moderately

with a decrease of superconducting $T_c$ around 0.5 K. The carrier density obtained from the hall measurement at 2 K is 6.55 × $10^{13}$ $cm^{-2}$ which evidences loss of carriers in the 2DEG due to the re-oxygenation of the sample. The electron mobilities along $[\bar{1}\bar{1}2]$ and $[1\bar{1}0]$ directions are 111 $cm^2V^{-1}s^{-1}$ and 33 $cm^2V^{-1}s^{-1}$, respectively.

## XPS measurements:

We have performed x-ray photoelectron spectroscopy (XPS) measurements before and after depositing 3Å of Eu. In Fig. S2(a) Ta is only present in 5+ state suggesting that no oxygen vacancies are present in the pristine substrate. After deposition of 3Å of Eu (Fig. S2(b)), the XPS data suggests formation of oxygen vacancies as peaks corresponding to $Ta^{4+}$ as well as $Ta^{2+}$ are evolved. According to the fitting 4.8% of $Ta^{5+}$ are reduced to $Ta^{4+}$ state and 1.8% even further to $Ta^{2+}$ state. Although, the presence of $Ta^{2+}$ could be arguable as it is possible to achieve similar quality fits without the $Ta^{2+}$ contribution. However, the presence of $Ta^{4+}$ peaks are prominent and thus confirms the formation of the oxygen vacancies.

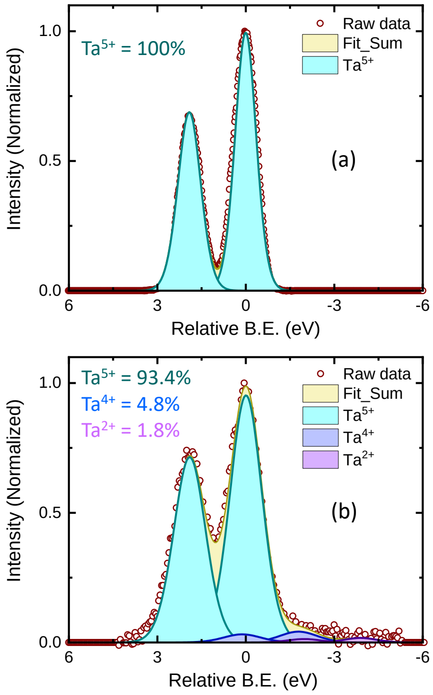


FIG. S2. XPS data and corresponding fits at Ta 4f edge for (a) KTO 111 pristine substrate and (b) after 3Å of Eu deposition showing formation of oxygen vacancies.

## LEED measurements:

Fig. S3 (a) and (b) show the low energy electron diffraction (LEED) patterns collected before and after Eu deposition, respectively. The pattern for the KTO (111) substrate shows sharp diffraction spots corresponding to a hexagonal symmetry as well as triangular symmetry. The hexagonal lattice attests the 111 planes of the KTO crystal. We have marked the hexagonal symmetry of the KTO (111) substrate on the image. Along with the hexagonal symmetry, triangular symmetry is also present in the substrate which may arise due to the surface reconstruction happened during the pre-annealing of the substrate at 500°C. However, after Eu deposition some bright spots were observed in the LEED image having triangular symmetry and not the original hexagonal symmetry of the substrate.

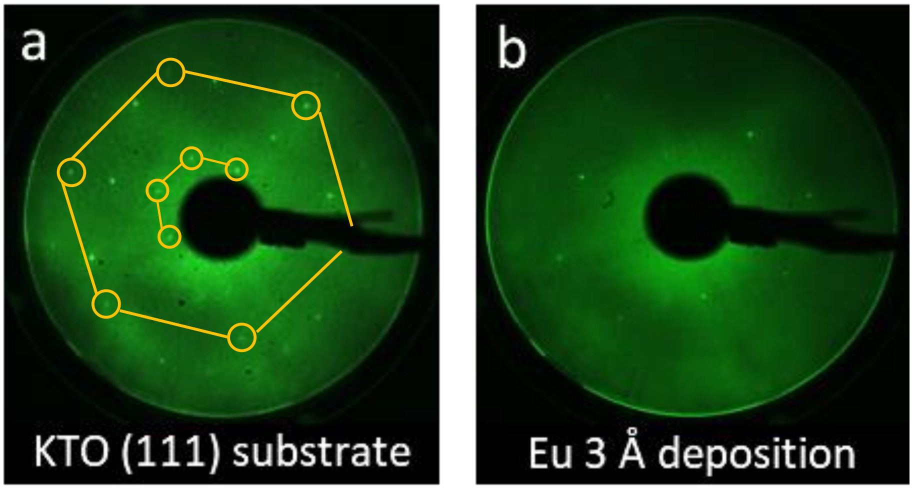


FIG. S3: LEED patterns for (a) the KTO (111) substrate after annealing at 500 °C and (b) after depositing 3 Å of Eu at 300 °C. The hexagonal patterns of the substrate having (111) surface are marked with yellow lines.

**ARPES measurements:**

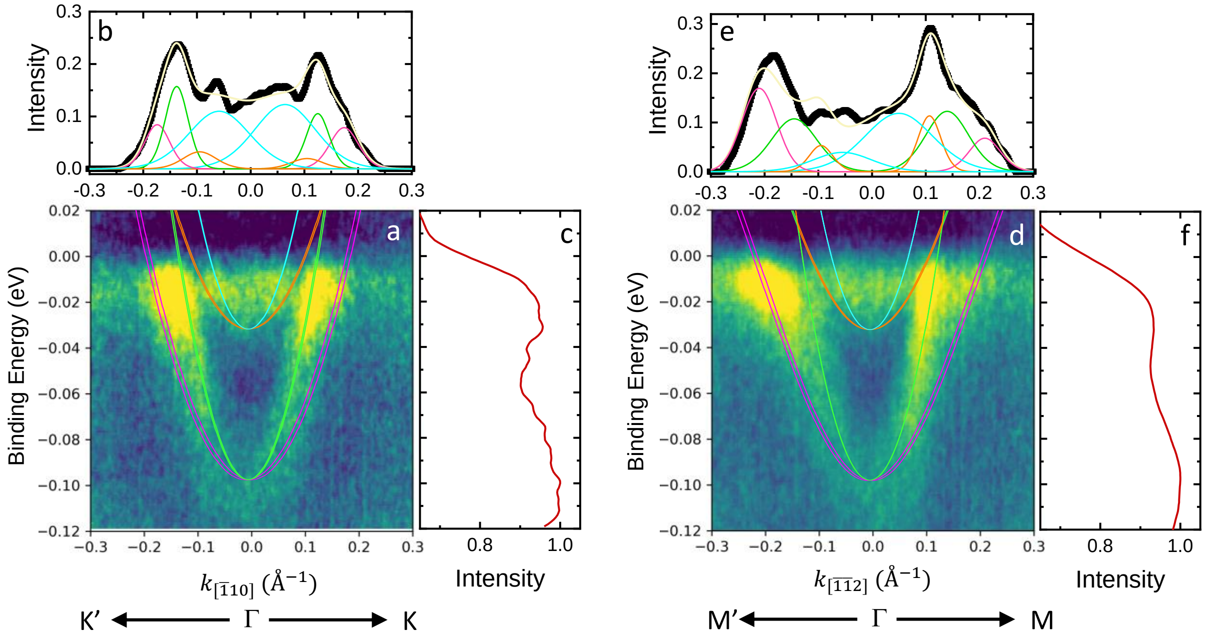


FIG. S4. Band dispersion of Eu/KTO (111) 2DEG measured by ARPES along high symmetry directions (a) Γ - K and (d) Γ - M. The tight-binding fits of the band structure are overlaid to the data where a specific color is associated with each pair of bands. Momentum distribution curves (MDC) at $E_F$ are shown in (b) for Γ - K and in (e) for Γ - M directions. To resolve the band positions both MDCs are fitted with 8 peaks corresponding to 4 band pairs. The color of the fitted lines of MDCs are equivalent to the color of the TB fitted bands. Energy distribution curves (EDC) at Γ are shown in (c) and (f). The positions of the bottom of the bands are determined from the peaks in the EDCs.

The momentum distribution curves (MDCs) near $E_F$ along K' – Γ – K and along M' – Γ – M are plotted in Fig. S4(b) and (e). To identify the $k_F$ values for the pink, green, orange and blue bands we have fitted the MDC with eight Gaussian peaks, two per band (one along Γ – K and one along Γ – K’). For a given band (say the pink) we have set the position of the two peaks to be symmetric with respect to Γ and to have the same full width at half maximum. For K’ – Γ – K, the peaks from the pink and green bands are easily resolved and their positions in Fig. S4(b) match well with the $k_F$ values from Fig. S4(a). The fit also captures well the position of the blue and orange bands. For M’ - Γ - M, the agreement is good for the pink band and satisfactory for the blue and orange bands, but less so for the green band. We have tried to vary the parameters in our tight-binding model, notably the hopping constants, in order to obtain a better fit in particular for the green band. However, we could not find a better set of parameters: increasing $k_F$ along Γ - M for the green band would imply increasing $k_F$ for all the band pairs and consequently impact the fits along Γ - K direction. Nevertheless, our analysis of the MDCs suggests that the agreement between our data and our TB fits is generally good and able to capture the main features of the band structure of our KTO (111) 2DEG. Further, the bottom of the bands for the TB fits are determined from the maxima of the energy distribution curves (EDC) shown in Fig. S4(c) and (f).

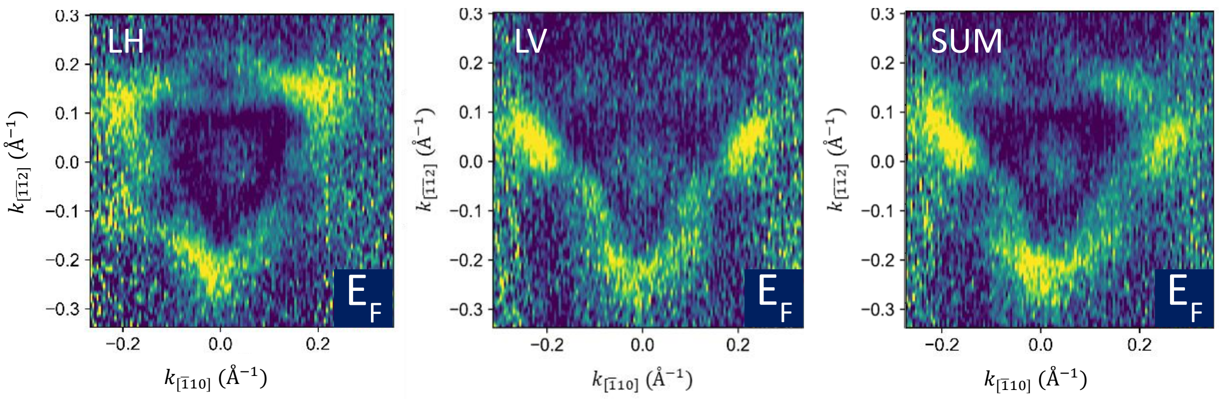


FIG. S5: Constant energy maps at E = $E_F$ measured with linear horizontal (LH) and linear vertical (LV) polarizations. The rightmost image shows the sum of these two images to obtain the full picture of the Fermi surfaces at the Fermi energy.

We have also measured our sample using linear vertical (LV) polarization of the photons. Fig. S5 shows the Fermi surface at E = $E_F$ for LH, LV polarizations and their sum. However, due to technical problems (tilt of the sample) we observed intensity only in one half of the images. Therefore, we did not use them in fitting the band structure and also didn’t draw any conclusion from these LV polarization images.
